# Supplementary material for: ActiveEA: Active Learning for Neural Entity Alignment
Source: arXiv:2110.06474 source file (2021-10-13)
Supplement: Supplementary file 1 [file appendix.tex]

%\newpage
%
%\section{Additional Reproducibility Information}
%
%% Computing infrastructure:
%Our experiments were run on a GPU cluster.
%We allocated 50G memory and 1 32GB nVidia Tesla V100 GPU for each job on 15K data, and 100G memory for each job on 100K data.
%%
%The training and evaluation of ActiveEA took approximately 3h with Alinet on 15K data, 10h with BootEA on 15K data, 10h with RDGCN on 15K data, and 48h with Alinet on 100K data.
%Most baseline strategies took less time than ActiveEA on the same dataset except \textit{betweenness} on 100K data, which took more than 48h.
%%
%We applied grid search for setting $\alpha$ and $N$ (shown in Sec.~\ref{sec:sensitivity_of_parameter}).
%Hyper-parameters of the bachelor recognizer were chosen based on the settings of OpenEA and our own random search.
%%we searched these hyper-parameters with few ($<5$) runs.
%
